# Supplementary material for: Finding hidden-feature depending laws inside a data set and classifying it using Neural Network
Source: arXiv:2101.10427 source file (2021-01-25)
Supplement: Supplementary file 1 [file appendix.tex]

\section{Table of Symbols}

\begin{center}
 \begin{tabular}{||c c||} 
 \hline
 Symbol &Interpretation\\ [0.5ex] 
 \hline\hline
 $\freeEn$ & Free Energy  \\ 
 \hline
 $\stress$ & Cauchy's Stress  \\ 
 \hline
$\genF$ & Generalized Forces  \\ 
 \hline
$\genV$ & Generalized Velocity  \\ 
 \hline
$\Temp$ & Absolute Temperature  \\ 
 \hline
$\SpEnt$ & Specific Entropy  \\ 
 \hline
$\IntEn$ & Internal Energy  \\ 
 \hline
$\den$ & Density  \\
 \hline
$\strain$ & Strain Deformation Tensor  \\  
 \hline
$\strainRate$ & Strain Rate Tensor  \\  
 \hline
$\heatflux$ & Heat Flux  \\
 \hline
$\diss$ & Specific Dissipation \\
 \hline
$\pot$ & Potential Function  \\
 \hline
$\enSource$ & Energy Souce per Unit mass  \\    
 \hline
\end{tabular}
\end{center}
